# Supplementary material for: Detection of nonlinearity, discontinuity and interactions in generalized regression models
Source: arXiv:2310.20409 source file (2023-10-31)
Supplement: Supplementary file 1 [file Supplement.pdf]

# SUPPLEMENTARY MATERIAL

## Basic Algorithm

A detailed description of the DENDI algorithm given multiple continuous covariates $x_1, \ldots, x_p$ is given below:

**Step 1:**

(a) *Evaluate the null model:* Fit the null model with predictor function

$$\eta(\boldsymbol{x}_i, \boldsymbol{z}_i) = \beta_0 + \boldsymbol{\delta}^\top \boldsymbol{z_i} \ ,$$

on each of the $n$ LOOCV training data sets and calculate the log-likelihood of the $n$ fitted models on the respective test observations. Calculate the average predicted log-likelihood value $p\ell^{[0]}$ and the standard error $SE^{[0]}$.

(b) *Initialization:* Set $j = 1$, $E_l = \{\}$ and $E_p = \{\}$.

(c) *Evaluate the two modeling alternatives:*

1) *Linear model:* Fit the linear model with predictor function

$$\eta(\boldsymbol{x}_i, \boldsymbol{z}_i) = \beta_0 + \beta_j \, x_{ij} + \boldsymbol{\delta}^\top \boldsymbol{z_i}$$

on each of the $n$ LOOCV training data sets and calculate the average predicted log-likelihood value $p\ell_j^{[l]}$ on the test observations.

2) *Piecewise constant model:* Fit the piecewise constant model with predictor function

$$\eta(\boldsymbol{x}_i, \boldsymbol{z}_i) = \beta_0 + \gamma_1 \, I(x_{ij} > c_j) + \boldsymbol{\delta}^\top \boldsymbol{z_i}$$

on each of the $n$ LOOCV training data sets and calculate the average predicted log-likelihood value $p\ell_j^{[p]}$ on the test observations.

(d) *Select effect:* Set

$$s = \underset{e \in \{l,p\}}{\arg\max} \, p\ell_j^{[e]}.$$

Then, if $p\ell_j^{[s]} > p\ell^{[0]} + SE^{[0]}$, set $E_s = E_s \cup \{j\}$ .

(e) *Update index:* If $j < p$, set $j = j + 1$ and continue with (1c). Otherwise, continue with step 2.

**Step 2:**

(a) *Evaluate the model based on step 1:* Fit the multivariable model with all previously selected effects, i.e.

$$\eta(\boldsymbol{x}_i, \boldsymbol{z}_i) = \beta_0 + \sum_{l \in E_l} \beta_l \, x_{il} + \sum_{l \in E_p} \gamma_l \, I(x_{il} > c_l) + \boldsymbol{\delta}^\top \boldsymbol{z_i}$$

on each of the $n$ LOOCV training data sets and calculate the average predicted log-likelihood value $p\ell^{[1]}$ and the standard error $SE^{[1]}$.

(b) *Initialization:* Set $j = 1, E_a = \{\}, E_m = \{\}$ and $E_t = \{\}$.

(c) *Evaluate the three modeling alternatives:*

1) *Additive combination:* If $j \in E_l$ or $j \in E_p$, fit the additive model with predictor function

$$\eta(\boldsymbol{x}_i, \boldsymbol{z}_i) = \beta_0 + \beta_j\, x_{ij} + \gamma_j\, I(x_{ij} > c_j) + \sum_{l \in E_l \setminus \{j\}} \beta_l\, x_{il} + \sum_{l \in E_p \setminus \{j\}} \gamma_l\, I(x_{il} > c_l) + \boldsymbol{\delta}^\top \boldsymbol{z_i}$$

on each of the $n$ LOOCV training data sets and calculate the average predicted log-likelihood value $p\ell_{jj}^{[a]}$ on the test observations.

2) *Multiplicative combination:* If $j \in E_l$, fit the multiplicative model with predictor function

$$\eta(\boldsymbol{x}_i, \boldsymbol{z}_i) = \beta_0 + \beta_{j1}\, x_{ij} + \beta_{j2}\, I(x_{ik} > c_k)(x_{ij} - c_k) + \sum_{l \in E_l \setminus \{j\}} \beta_l\, x_{il} + \sum_{l \in E_p} \gamma_l\, I(x_{il} > c_l) + \boldsymbol{\delta}^\top \boldsymbol{z_i}$$

for $k = j$ and with predictor function

$$\eta(\boldsymbol{x}_i, \boldsymbol{z}_i) = \beta_0 + \beta_{j1}\, x_{ij} + \beta_{j2}\, I(x_{ik} > c_k) x_{ij} + \sum_{l \in E_l \setminus \{j\}} \beta_l\, x_{il} + \sum_{l \in E_p} \gamma_l\, I(x_{il} > c_l) + \boldsymbol{\delta}^\top \boldsymbol{z_i}$$

for all $k \in \{1, \ldots j-1, j+1, \ldots p\}$ on each of the $n$ LOOCV training data sets and evaluate the $n \times p$ models on the respective test observations. Calculate the average predicted log-likelihood values $p\ell_{jk}^{[m]}$.

3) *Tree-structured model:* If $j \in E_p$, fit the tree-structured model with predictor

$$\eta(\boldsymbol{x}_i, \boldsymbol{z}_i) = \beta_0 + \gamma_{jr}\, I(x_{ij} > c_j) + \gamma_{j\ell}\, I(x_{ij} \le c_j \wedge x_{ik} > c_k) \sum_{l \in E_l} \beta_l\, x_{il} + \sum_{l \in E_p \setminus \{j\}} \gamma_l\, I(x_{il} > c_l) + \boldsymbol{\delta}^\top \boldsymbol{z_i}$$

for all $k \in \{1, ..., p\}$ on each of the $n$ LOOCV training data sets and evaluate the $n \times p$ models on the respective test observations. Note that the selection of the optimal split point by TSVC also allows that the second split is in $\{x_{ij} > c_j\}$ (see Equation (**??**)), which is omitted here. Calculate the average predicted log-likelihood values $p\ell_{jk}^{[t]}$.

(d) *Select effect:* If $j \in E_l$ or $j \in E_p$, set

$$(s, o) = \underset{(e,k) \in H}{\arg\max}\, p\ell_{jk}^{[e]}$$

with

$$H = \begin{cases} \{(a, j), (m, 1), ..., (m, p)\} & \text{if } j \in E_l \\ \{(a, j), (t, 1), ..., (t, p)\} & \text{if } j \in E_p\,. \end{cases}$$

Then, if $p\ell_{jo}^{[s]} > p\ell^{[1]} + SE^{[1]}$, set $E_s = E_s \cup \{(j, o)\}$, $E_l = E_l \setminus \{j\}$ and $E_p = E_p \setminus \{j\}$.

(e) *Update index:* If $j < p$, set $j = j + 1$ and go to (2c). Otherwise, terminate the algorithm.

## Additional results of the simulation study

Table S1: Results of the simulation study (scenario 2). Summary statistics of the split points selected by the algorithm when fitting the piecewise constant model in the setting with low noise ($\sigma = 1$) and large sample size ($n = 800$).

| | Summary statistics | | | | | |
|---|---|---|---|---|---|---|
| | $c_{min}$ | $c_{0.25}$ | $c_{med}$ | $\overline{c}$ | $c_{0.75}$ | $c_{max}$ |
| Split points | -0.12 | -0.04 | -0.01 | -0.01 | 0.03 | 0.15 |

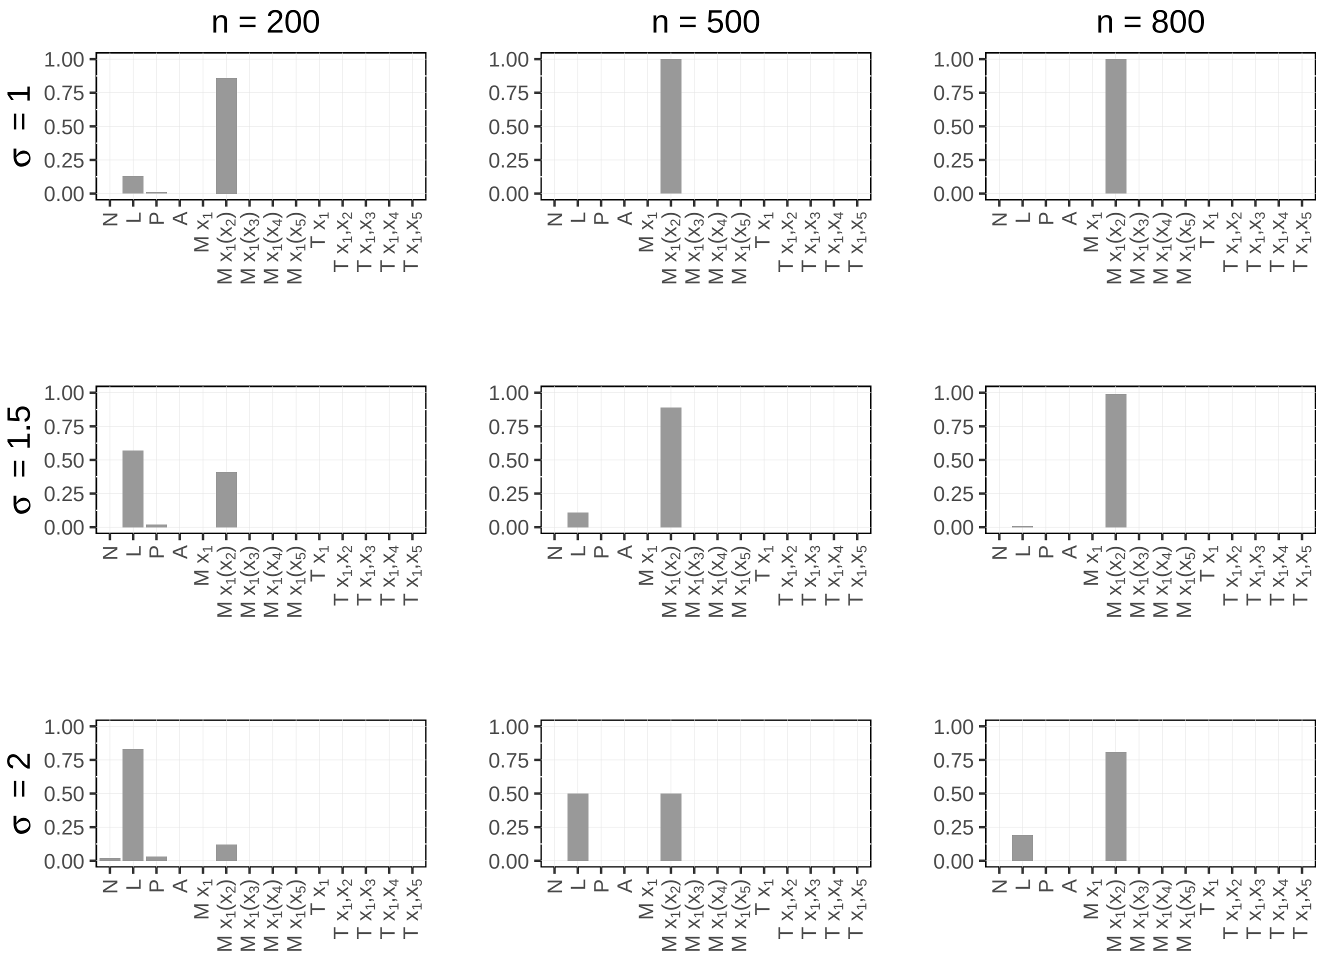


Figure S1: Results of the simulation study (multivariable scenario). The figure shows the proportions of simulation runs in which the different modeling alternatives (N, L, P, A, M $x_1$, M $x_2$, M $x_3$, M $x_4$, M $x_5$, T $x_1$, T $x_2$, T$x_3$, T $x_4$, T $x_5$) were selected by the algorithm for modeling $x_1$. The multiplicative effect M and the tree-structured effect T can either be univariable (M $x_1$, T $x_1$) or bivariable. Selection rates for sample sizes $n \in \{200, 500, 800\}$ (columns) and standard deviations $\sigma \in \{1, 1.5, 2\}$ (rows) are presented.

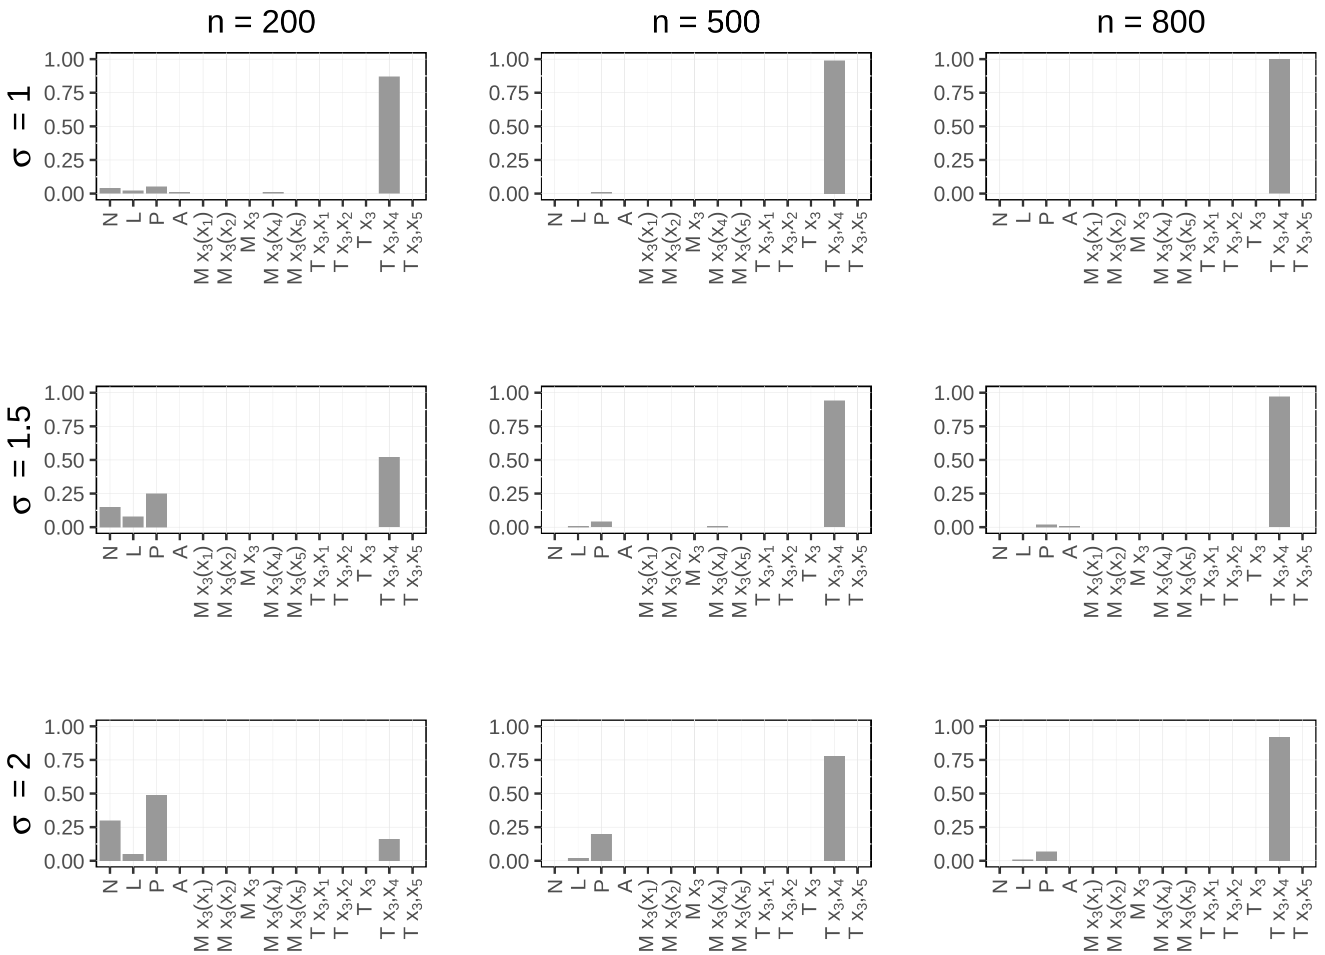


Figure S2: Results of the simulation study (multivariable scenario). The figure shows the proportions of simulation runs in which the different modeling alternatives (N, L, P, A, M $x_1$, M $x_2$, M $x_3$, M $x_4$, M $x_5$, T $x_1$, T $x_2$, T$x_3$, T $x_4$, T $x_5$) were selected by the algorithm for modeling $x_3$. The multiplicative effect M and the tree-structured effect T can either be univariable (M $x_3$, T $x_3$) or bivariable. Selection rates for sample sizes $n \in \{200, 500, 800\}$ (columns) and standard deviations $\sigma \in \{1, 1.5, 2\}$ (rows) are presented.

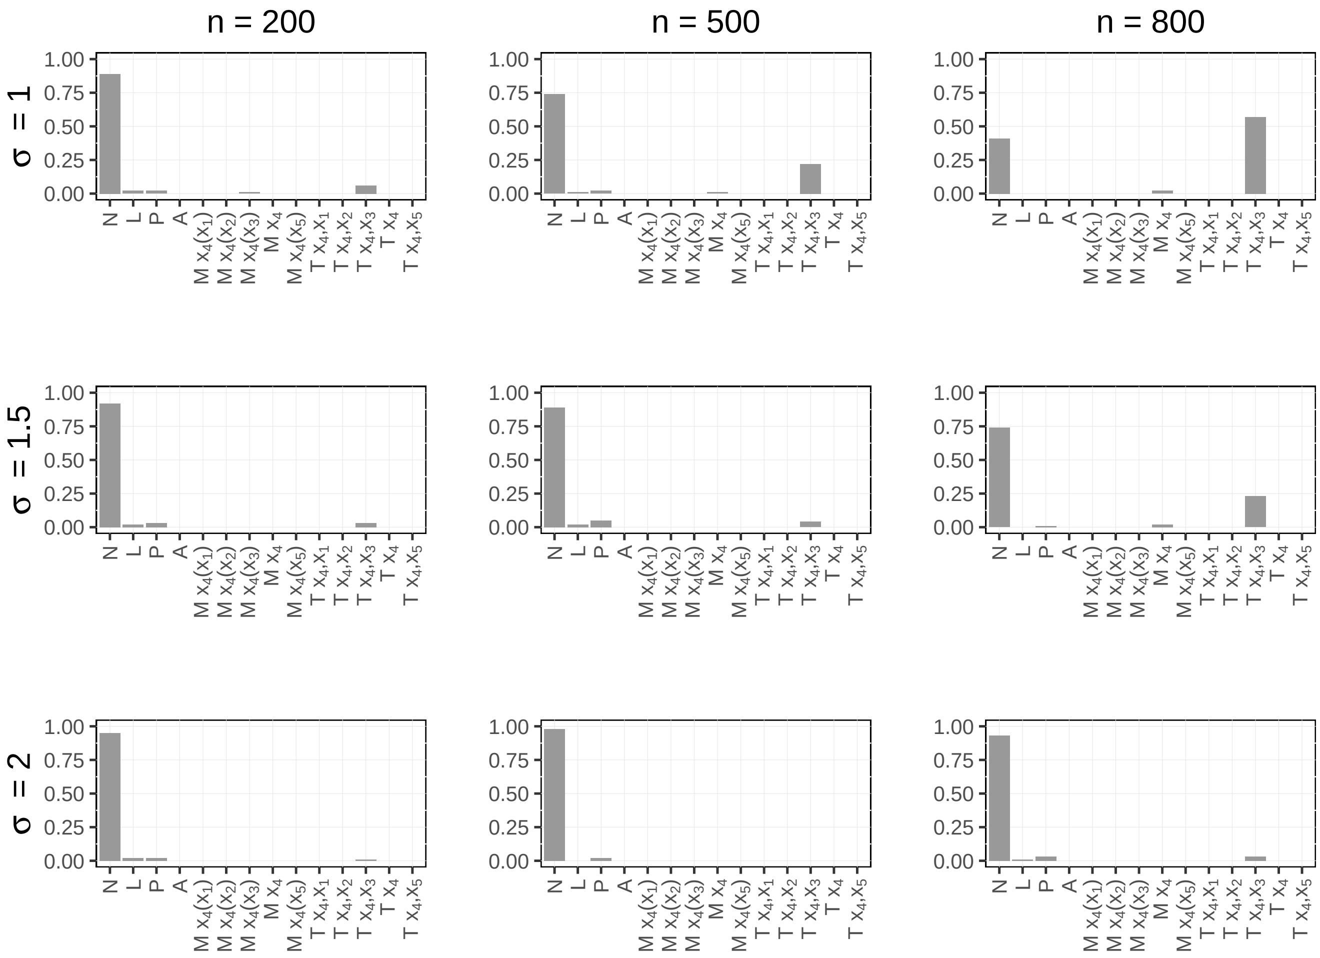


Figure S3: Results of the simulation study (multivariable scenario). The figure shows the proportions of simulation runs in which the different modeling alternatives (N, L, P, A, M $x_1$, M $x_2$, M $x_3$, M $x_4$, M $x_5$, T $x_1$, T $x_2$, T$x_3$, T $x_4$, T $x_5$) were selected by the algorithm for modeling $x_4$. The multiplicative effect M and the tree-structured effect T can either be univariable (M $x_4$, T $x_4$) or bivariable. Selection rates for sample sizes $n \in \{200, 500, 800\}$ (columns) and standard deviations $\sigma \in \{1, 1.5, 2\}$ (rows) are presented.

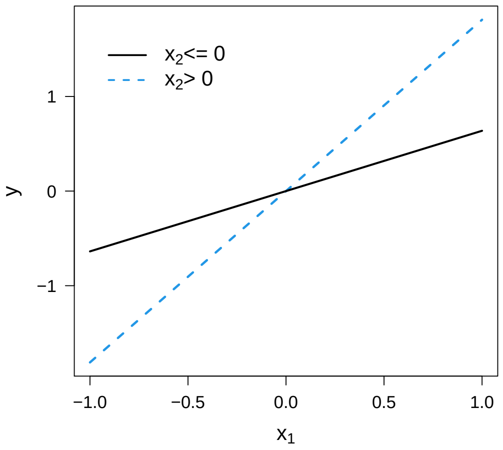


(a) Effect of $x_1$ modified by $x_2$

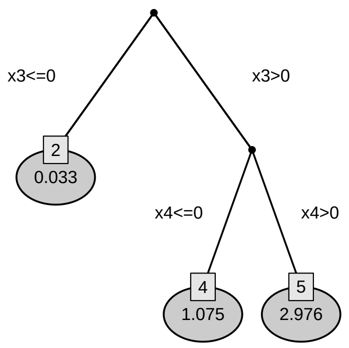


(b) Interaction between $x_3$ and $x_4$

Figure S4: Results of the simulation study (multivariable scenario). Estimated effects of a model that was specified according to the results of DENDI for an exemplary data set with $n = 800$ and $\sigma = 1$ (all effects where correctly identified). The left panel (a) visualizes the estimated linear effect of $x_1$ modified by $x_2$, the right panel (b) the tree-structured interaction between $x_3$ and $x_4$.

## Additional results of the application to the GCKD study data

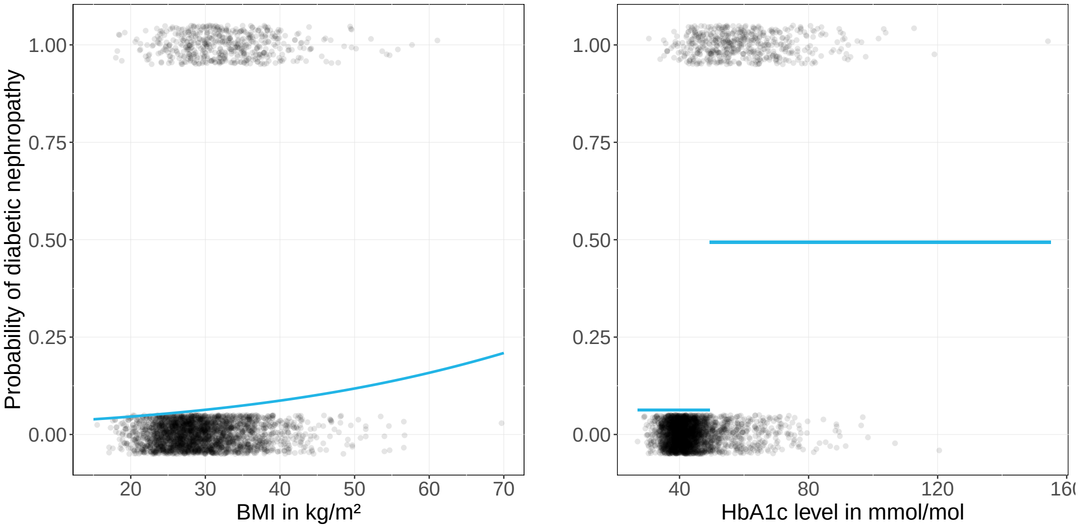


(a) Effect of BMI

(b) Effect of HbA1c level

Figure S5: Analysis of the GCKD study data. Estimated effects of a multivariable model for diabetic nephropathy based on the results of DENDI. The estimates correspond to exemplary patients with mode values for sex (male), education (lower education) and employment status (retired), and median values for HbA1c level (42.7 mmol/mol) and BMI (29.1 kg/m$^2$), respectively. The left panel (a) illustrates the adjusted effect of BMI on the conditional probability of suffering from diabetic nephropathy, the right panel (b) illustrates the adjusted piecewise constant effect of HbA1c level. The observed outcome values are marked by jittered black dots.

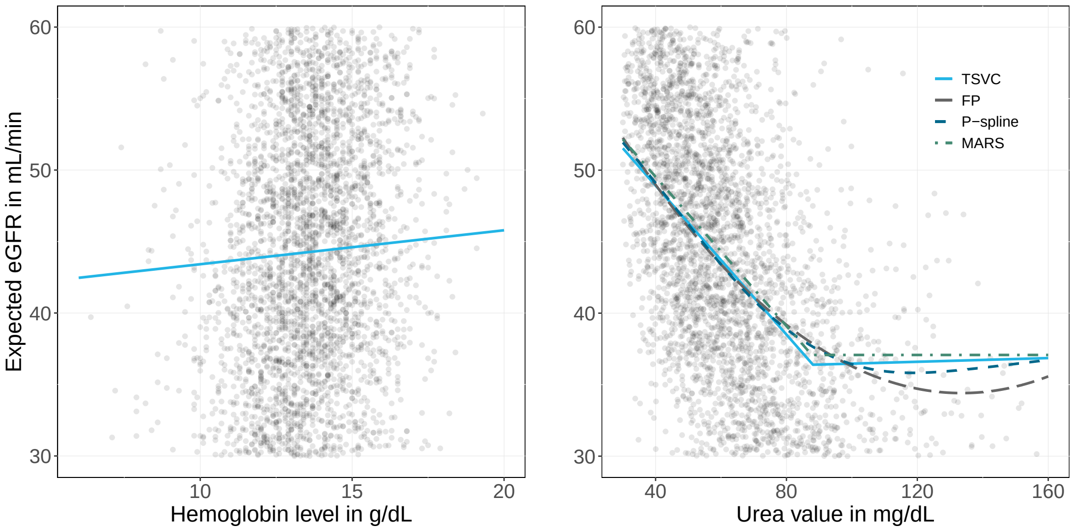


(a) Effect hemoglobin level

(b) Effect of urea

Figure S6: Analysis of the GCKD study data. Estimated effects of a multivariable analysis for eGFR based on the results of DENDI. The estimates correspond to exemplary patients with mode values for education (lower education) and employment status (retired), and median values for urea (57.9 mg/dL) and hemoglobin level (13.6 g/dL), respectively. The left panel (a) illustrates the adjusted linear effect of hemoglobin level on the expected eGFR, the right panel (b) illustrates the adjusted effects based on more complex modeling alternatives (TSVC, fractional polynominals (FP), P-Spline and MARS) for the effect of urea, where a varying linear effect was detected. The observed outcome values are marked by black dots.
